# Supplementary material for: Unifying Short and Long-Term Tracking with Graph Hierarchies
Source: arXiv:2212.03038 source file (2023-03-30)
Supplement: Supplementary file 1 [file additional_experiments.tex]

%!TEX root = ../../supplementary_material.tex
%\section{Additional Experiments}\label{sec:experiments_supplementary}






\iffalse
\subsection{Analysis on maximum temporal edge distance}
\modelname is capable of processing clips of arbitrary length but we construct graphs with a maximum temporal edge distance of 150 frames as we experimentally found that this covers the majority of long-term association cases. In Figure~\ref{fig:ablation_aplift}, we visualize the maximum frame gaps within trajectories as a histogram on the MOT17 training set when public detections are associated by an oracle. A vast majority of the trajectories (more than 98\%) can be constructed without an error with a clip size of 150 frames, and gains diminish for higher frame distances. In addition, we report the cross-validation scores obtained by our model with different maximum temporal edge distance parameters in Figure~\ref{fig:clipsize_idf1}. We observe that processing larger clips improves the results up to 150 frames but scores stagnate after this point. Overall, we experimentally found 150 frames to be a good trade-off between performance, memory requirements, and training speed. 

\begin{figure}
\centering
\includegraphics[width=\columnwidth]{supplementary/figures/mot17analysis.png}
\caption{Histogram of maximum frame distance of trajectories constructed by an oracle on MOT17 training set.}
\label{fig:ablation_aplift}
\end{figure}

\begin{figure}
\centering
\includegraphics[width=\columnwidth]{supplementary/figures/clipsize_idf1.png}
\caption{Scores reached by our model with different maximum temporal edge distance parameters.}
\label{fig:clipsize_idf1}
\end{figure}

\fi


\iffalse
\subsection{Memory requirement and hierarchy levels}

Our graph hierarchy significantly reduces the number of edges in a graph  and further mitigates the label imbalance between correct and incorrect trajectory hypotheses, as we showed in the Figure 4a of the main paper. 
Consequently, having fewer edges in graphs results in lower memory requirements to train models. We further quantify this phenomenon by reporting the upper bound IDF1 score and peak training memory with a varying number of hierarchical levels in Figure~\ref{fig:memory}. Each data point is obtained by setting different K values while pruning during graph construction. We observe that our hierarchy drastically reduces the peak training memory requirements. Specifically, a non-hierarchical configuration with a single level achieves 55 IDF1 with approximately 20 GB memory, while the models with four and five levels reach 81 IDF1 with one-fourth of the memory requirement.  
\begin{figure}
\centering
\includegraphics[width=\columnwidth]{supplementary/figures/memoryv2.png}
\caption{Upper bound IDF1 score with respect
to peak training memory. GPU limit is given
for a single Quadro RTX 8000 GPU.}
\label{fig:memory}
\end{figure}
\fi

\iffalse
\begin{figure}
\centering
\includegraphics[width=\columnwidth]{supplementary/figures/ablation_localmot.pdf}
\caption{Temporal analysis of tracking performance with LocalMOT.}
\label{fig:localmot}
\end{figure}


\subsection{Temporal analysis of tracking performance} 
We perform a temporal analysis on our model with a different number of hierarchy levels (\blocknameplural) as well as MPNTrack to outline how different aspects of tracking benefit from our hierarchy in Figure~\ref{fig:localmot}. For this, we use LocalMOT~\cite{localmot} which restricts IDF1 computation to a finite temporal horizon and breaks down how a tracker's performance evolves from short-term to long-term. We observe monotonic improvements in association performance across all temporal horizons with models with more hierarchy levels. Especially in large temporal horizons, corresponding to long-term association cases, we observe a significant performance increase compared to MPNTrack, which indicates that we especially improve long-term tracking with our hierarchical method.

\input{tables/supplementary/ablation_frames} 

\subsection{Clip sizes partition configuration} Our graph hierarchies are based on a recursive partition of a video into clips. In order to get the most out of our proposed graph hierarchies, their corresponding clip length configurations needs to be carefully designed. 
Intuitively, clips should grow in a progressive manner, so that the tracklet-merging workload is evenly distributed among hierarchy levels. In Tab. \ref{table:ablation_frames}, we explore several variations of our best configuration. All variations consist of 4 levels operating over a clip with 150 frames. In rows \#2 and \#3, the small windows in the early layers focus mostly on short-term associations, and the final merging of tracklets is relatively aggressive.
The full potential of the hierarchy cannot be exploited in this configuration: later levels operate over relatively short tracklets and therefore have less robust association cues. At the same time, they attempt to merge tracklets from an increased number of clips, thereby increasing the complexity of their task.
%
In contrast, rows \#4 and \#5 start from large clips and quickly consider tracklets spanning over all frames at once. Since at the first level we cannot compute tracklet-level features, \eg based on motion, the model is more prone to errors. These errors are then propagated to later layers and cannot be recovered.
%
As we can see in row \#1, our configuration yields better results, highlighting the importance of following a more balanced merging sequence. 





\input{tables/supplementary/ablation_appearance.tex}
\subsection{Appearance features} As we observed in Figure 4c of the main paper, appearance plays the largest role among all feature sources. In Table \ref{table:appearance}, we further investigate alternative ways to encode track-level appearance. Notably, using appearance embeddings from the closest detections among tracklets instead of average tracklet-level embeddings yields a significant decrease of over 5 IDF1. This highlights the importance of exploiting the entire set of appearance embeddings over tracklets. Lastly, aggregating embeddings with a max operation, instead of averaging them, yields a modest decrease of 1.5 IDF1.  
\fi

\iffalse
\subsection{Different ReID model} 
Our method inherits the GNN architecture of MPNTrack~\cite{mpntrack}, but we use a different reID model as their model is trained on a retracted dataset. Specifically, instead of ResNet50~\cite{he2016deep}, we use a ResNet50-IBN~\cite{ibn} variant, following \cite{lpc}, pretrained on MSMT17~\cite{Wei2018PersonTG}, an extension of Market-1501\footnote{The model is publicly available at \url{https://github.com/JDAI-CV/fast-reid/blob/master/MODEL_ZOO.md}}. We do this in an attempt to match the reID performance of \cite{mpntrack}, without resourcing to withdrawn datasets. Note that MPNTrack~\cite{mpntrack} trained its model on three different datasets: Market-1501~\cite{Zheng2015ScalablePR}, CUHK03~\cite{cuhk}, and \textit{the currently retracted DukeMTC~\cite{Ristani2016PerformanceMA}}. Instead, we use a single public dataset \cite{Wei2018PersonTG}. In Table \ref{table:reid}, we report MOT17 cross-validation results using our reID model and the one used by \cite{mpntrack}. We observe that our reID model performs moderately worse. Despite using a clearly worse reID model, our overall approach still outperforms MPNTrack~\cite{mpntrack} by 6.9 IDF1 on the MOT17 test set. These results further highlight that our improvements are due to our main contributions.

\fi


\iffalse
\subsection{Extended benchmark results on MOTChallenge with public detections}
\input{tables/supplementary/extended_public.tex}

MOTChallenge presents a public setting in which object detections are provided to emphasize data association performance during evaluation. In the public setting, it is a common practice among published methods to refine the public detections of the MOTChallenge~\cite{tracktor, li2022learning, mpntrack, lift, aplift, gmt, lpc, centertrack, tmoh, bytetrack} with  local tracking schemes that enable adding additional boxes~\cite{ centertrack, tracktor, tmoh, bytetrack}. These processing schemes have a large impact on the detection quality and the overall tracking scores. 

In the main paper, we reported public setting results with the Tracktor-based refinement as it is the most commonly used one. To compare our method with a wider range of trackers, in Table~\ref{table:motcha_public} we report results with an additional processing scheme and show further improvements over methods using alternative preprocessing schemes as well. Specifically, we significantly outperform the state-of-the-art by +3.4 IDF1 and +2.4 HOTA on MOT17 and +3.1 IDF1 and +2.0 HOTA on MOT20 while using the same set of detections.

\fi





% \begin{figure}
% \centering
% \includegraphics[width=\columnwidth]{supplementary/figures/mot17-byte.png}
% \caption{\TODO{Byte065 detection based max trajectory gap on MOT17.} \orc{MOST LIKELY WE WILL DROP THIS!}}
% \label{fig:ablation_byte}
% \end{figure}
