# Supplementary material for: Unifying Short and Long-Term Tracking with Graph Hierarchies
Source: arXiv:2212.03038 source file (2023-03-30)
Supplement: Supplementary file 2 [file ablation_appearance.tex]

%!TEX root = ../../main.tex
\begin{table}
\center
\tabcolsep=0.11cm
    \resizebox{\columnwidth}{!}{
    \begin{tabular}{l l c c c c c c }
     \toprule
    Appearance representation & IDF1 $\uparrow$ & HOTA $\uparrow$ & MOTA $\uparrow$ \\ [0.5ex] 
     \midrule
     
     Closest obj. detection & 70.8 &  62.4 & 68.0 \\
     Track-Max & 74.5 &  64.8 &  68.3 \\
     Track-Avg & 76.0 & 65.8  &  68.6\\

     \midrule

    \end{tabular}}

\caption{Effect of different appearance representations.}
\label{table:appearance}
\end{table}
