# Supplementary material for: Unifying Short and Long-Term Tracking with Graph Hierarchies
Source: arXiv:2212.03038 source file (2023-03-30)
Supplement: Supplementary file 3 [file ablation_frames.tex]

\begin{table}
\center
\tabcolsep=0.11cm
    \resizebox{\columnwidth}{!}{
\begin{tabular}[b]{c l l c c c c c c c c}
     \toprule
     \# & Strategy & Clip sizes & IDF1 $\uparrow$  & HOTA $\uparrow$ & MOTA $\uparrow$ \\ [0.5ex] 
     
     \midrule
     1 & Balanced (Ours) & 5-25-75-150  & 76.0 &   65.8 & 68.6 \\
     
    %  \midrule 
    %  Balanced & 5-25-75 & -- & 72.9 & 67.6 & -- & -- & -- \\
    %  Balanced & 5-25 & -- & 67.1 & 66.7 & -- & -- & -- \\
    %  Balanced & 5 & -- & 62.0 & 66.3 & -- & -- & -- \\
     
     \midrule
     2 & Short Term & 2-6-30-150 & 73.0 & 63.7 & 68.2 \\
     3 & Short Term & 5-10-30-150 & 74.0 & 64.4 & 68.0\\
     4 & Long Term & 25-75-150-150 & 66.2  & 59.1 & 60.6\\
     5 & Long Term & 50-150-150-150 & 59.6 & 54.3 & 48.8\\
     \midrule
    \end{tabular}
    }

\caption{Clip sizes partition configuration.}
\label{table:ablation_frames}
\end{table}
