# Supplementary material for: Unifying Short and Long-Term Tracking with Graph Hierarchies
Source: arXiv:2212.03038 source file (2023-03-30)
Supplement: Supplementary file 5 [file ablation_pruning.tex]

%!TEX root = ../../main.tex
\begin{table}
\center
\tabcolsep=0.11cm
    \resizebox{\columnwidth}{!}{
    \begin{tabular}{l l c c c c c c }
     \toprule
     Level 1 sim. & Level 2-4 sim. & IDF1 $\uparrow$ & HOTA $\uparrow$ & MOTA $\uparrow$  & ID Sw. $\downarrow$ \\ [0.5ex] 
     \midrule
     App. & App. & 75.6 & 65.6 &  68.6  & 736 \\
     Pos. & App. & 75.6 &  65.6 &  68.5  &732 \\
     Pos. & App. + Motion & 76.0  & 65.8 &  68.6 & 706 \\
     \midrule

    \end{tabular}}

\caption{Effect of different edge pruning strategies. \TODO{Are we still using this?}}
\label{table:supp_pruning}
\end{table}
