# Supplementary material for: Unifying Short and Long-Term Tracking with Graph Hierarchies
Source: arXiv:2212.03038 source file (2023-03-30)
Supplement: Supplementary file 7 [file reid.tex]

%!TEX root = ../../main.tex
\begin{table}
\center
\tabcolsep=0.11cm
    \resizebox{\columnwidth}{!}{
    \begin{tabular}{l c c c c c c c }
     \toprule
    ReID model & Training data & IDF1 $\uparrow$ & HOTA $\uparrow$ & MOTA $\uparrow$ \\ [0.5ex] 
     \midrule
     
     ResNet50  & \cite{Zheng2015ScalablePR, cuhk, ristanieccvw2016} & \textcolor{red}{UPDATE} &  \textcolor{red}{UPDATE} &  \textcolor{red}{UPDATE} \\
     ResNet50-IBN & \cite{Wei2018PersonTG} & 77.6 &  66.7 &  68.9 \\

     \midrule

    \end{tabular}}

\caption{Effect of using \cite{mpntrack}'s original reID model (ResNet50 trained on 3 datasets) vs ours (ResNet50-IBN trained on a single dataset).}
\label{table:reid}
\end{table}
